# Supplementary material for: Resource Bounded Measure
Source: arXiv:1101.5455 source file (2012-01-31)
Supplement: Supplementary file 1 [file appendixc.tex]

\section{Proofs of Results}
\label{appendixc}
